# Supplementary material for: Multimodal Representation Alignment for Image Generation: Text-Image Interleaved Control Is Easier Than You Think
Source: arXiv:2502.20172 source file (2025-02-27)
Supplement: Supplementary file 1 [file X_suppl.tex]

\clearpage

\setcounter{page}{1}
\setcounter{section}{0}
\setcounter{figure}{0}
\setcounter{table}{0}

\maketitlesupplementary

\noindent The supplementary material is structured as follows:

\begin{itemize}[leftmargin=7.5mm]
\item Additional case studies in Section~\ref{supp:}.
\item Additional case studies in Section~\ref{supp:}.
\item Additional case studies in Section~\ref{supp:}.
\end{itemize}
